# Supplementary material for: Finite-Temperature Atomistic and Continuum Stress Fields of Coherent Precipitates with a Small Lattice Misfit
Source: arXiv:2411.03233 ancillary file (2024-11-05)
Supplement: Supplementary file 1 [file sup_mat.pdf]

# Supplementary Material for *Finite-Temperature Atomistic and Continuum Stress Fields of Coherent Precipitates with a Small Lattice Misfit*

Anas Abu-Odeh, James Warren

## 1. Fe-Cr Interatomic Potential

Table S1 below shows the coefficients of  $h(x)$  (the definition of this function is given in Ref. [1]) for the concentration-dependent embedded-atom method (CD-EAM) potential used in this study. The results in this work can be reproduced by taking the potential found in Ref. [2], and replacing the values in the very last line of the potential file with the values in Table S1. The newer CD-EAM parameterization results in a lower heat of mixing, as shown in Figure S1. The heat of mixing values were calculated at 0 K using 2000 atom body-centered cubic (BCC) supercells of random Fe-Cr solid solutions. For comparison, we also evaluate the heat of mixing using a two-band model (TBM)-EAM potential [3], and show the heat of mixing of the older CD-EAM potential [1, 4].

| poly. order | $h_0$    | $h_1$     | $h_2$    | $h_3$     | $h_4$    | $h_5$     | $h_6$    |
|-------------|----------|-----------|----------|-----------|----------|-----------|----------|
| 6           | 1.060308 | -1.182214 | 4.662174 | -9.059552 | 9.424173 | -5.122298 | 1.168842 |

Table S1: Polynomial coefficients for  $h(x)$  for the CD-EAM potential used in this study.

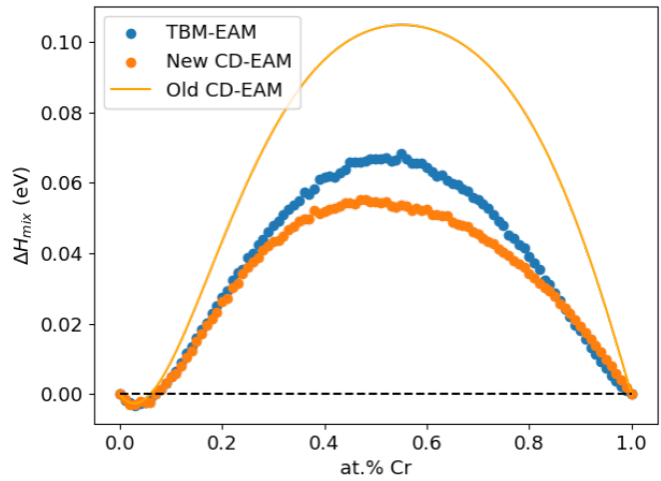

Figure S1: 0 K heat of mixing curves for random solid solutions of Fe-Cr on a BCC lattice using a TBM-EAM potential [3], an older CD-EAM potential [1, 4], and the new, reparameterized CD-EAM potential.

## 2. Kinetic Energy Contribution to Monte Carlo Moves

Here we show how the kinetic energy contribution in the Boltzmann distribution appears when constructing Monte Carlo (MC) moves in the semi-grand canonical (SGC) ensemble. If we describe a particular state by a set of three vectors,  $(\vec{p}, \vec{r}, \vec{\zeta})$ , which represent the momenta, positions, and chemical occupancy of each atom, respectively, then the probability of a state in a binary AB system is equal to:

$$P(\vec{p}, \vec{r}, \vec{\zeta}) = \exp(-\beta[K(\vec{p}) + U(\vec{r}, \vec{\zeta}) - \Delta\mu N_B])/Z \quad (\text{S1})$$

where  $\beta$  is equal to  $1/(k_B T)$ ,  $K(\vec{p})$  is the kinetic energy of the system,  $U(\vec{r}, \vec{\zeta})$  is the potential energy of the system,  $N_B$  is the total number of B atoms in the system, and  $Z$  is the partition function, which also acts as a normalization constant. The momentum degrees of freedom can be integrated out through:

$$\begin{aligned} P(\vec{r}, \vec{\zeta}) &= \int_{-\infty}^{\infty} P(\vec{p}, \vec{r}, \vec{\zeta}) d\vec{p} \\ &= \frac{\exp(-\beta[U(\vec{r}, \vec{\zeta}) - \Delta\mu N_B])}{Z} \int_{-\infty}^{\infty} \exp(-\beta K(\vec{p})) d\vec{p} \\ &= \frac{\exp(-\beta[U(\vec{r}, \vec{\zeta}) - \Delta\mu N_B])}{Z} \int_{-\infty}^{\infty} \exp\left(-\beta \sum_{i=1}^N \sum_{e=1}^3 \frac{p_{i,e}^2}{2m_i}\right) d\vec{p} \\ &= \frac{\exp(-\beta[U(\vec{r}, \vec{\zeta}) - \Delta\mu N_B])}{Z} \left(\frac{2\pi m_B}{\beta}\right)^{3N_B/2} \left(\frac{2\pi m_A}{\beta}\right)^{3(N-N_B)/2} \\ &= \frac{\exp(-\beta[U(\vec{r}, \vec{\zeta}) - \{\Delta\mu + \beta^{-1} \frac{3}{2} \ln(\frac{m_B}{m_A})\} N_B])}{Z} \left(\frac{2\pi m_A}{\beta}\right)^{3N/2} \end{aligned} \quad (\text{S2})$$

where  $N$  is the total number of atoms,  $e$  represents the different axes in Cartesian coordinates, and  $m_A/m_B$  is the mass of an A/B atom. Constructing a MC move where atomic species are flipped that satisfies detailed balance at equilibrium means accepting a flip attempt with a probability equal to the ratio of the probability of the trial state ( $\vec{\zeta}_t$ ) to that of the initial state ( $\vec{\zeta}_i$ ) (if this ratio is greater than 1, then the flip attempt is accepted):

$$\frac{P(\vec{r}_i, \vec{\zeta}_t)}{P(\vec{r}_i, \vec{\zeta}_i)} = \exp(-\beta[\Delta U(\vec{r}_i, \vec{\zeta}_i \rightarrow \vec{\zeta}_t) - \{\Delta\mu + \beta^{-1} \frac{3}{2} \ln(\frac{m_B}{m_A})\} \Delta N_B]). \quad (\text{S3})$$

This criterion has been used in previous studies [5, 6] and is implemented in the Para-GrandMC code [7].  $\Delta\mu$  as given above is equal to  $\partial f / \partial c$  at the given temperature, volume and composition of the system [8], and equal to  $\partial g / \partial c$  at the given temperature, pressure and composition of the system. However, the value of  $\tilde{\mu}$  as defined in the SGC MC implementation in the Large-scale Atomic/Molecular Massively Parallel Simulator (LAMMPS) is equal to the negative of the terms in the curly brackets in Eq. S3 as discussed in the next section.

### 3. Implementation of SGC and Variance-Constrained SGC MC in LAMMPS

In this work, we have modified the variance-constrained (VC)-SGC MC implementation in LAMMPS in order to determine the value of  $\Delta\mu$  ( $\mu_B - \mu_A$ ). The change is done to the line underlined in red in Figure S2 below. This snippet of code can be found in either the **fix\_sgcmc.cpp** file if using the package obtained from Ref. [9], or in the **fix\_sgcmc.cpp** file if using a current version of LAMMPS built with the MC package. Instead of initializing  $i = 1$  in the *for loop*, we initialize  $i = 2$  before building LAMMPS. This is because otherwise the contribution to determine the penalty for the outer MC acceptance loop, or the global trial move in Ref. [10], would be artificially too large due to a contribution related to the square of the change in the concentration of the host species. This contribution is not consistent with the discussion of this ensemble in Refs. [8, 10]. In principle, one could instead modify Eq. S5 below to account for this contribution, but we believe that the simple step of changing the code below also simplifies the post-processing steps.

```
// Perform outer MC acceptance test.
// This is done in sync by all processors.
double A = 0.0;
for (int i = 1; i <= atom->ntypes; i++) {
  A += deltaNGlobal[i] * deltaNGlobal[i];
  A += 2.0 * deltaNGlobal[i] * (speciesCounts[i] - (int)(targetConcentration[i] * atom->natoms));
}
```

Figure S2: Code snippet from a source file implementing the VC-SGCMC algorithm in LAMMPS.

We will use  $\Delta\mu$  to denote the chemical potential difference,  $\mu_B - \mu_A$ , and  $\tilde{\mu}$  to denote the input parameter used for SGC ensemble MC flips in LAMMPS. When evaluating the Metropolis criterion in LAMMPS, a flip is accepted with a probability of  $\min\{1, \exp(-\beta[\Delta U + \tilde{\mu}\Delta N_B])\}$ , where  $\beta$  is equal to  $1/(k_B T)$ ,  $\Delta U$  is the change in potential energy of the system when the flip is accepted, and  $\Delta N_B$  is the change in the number of B atoms. Due to the sign convention used in the above criterion as well as the neglect of the contribution of kinetic energy (discussed in the previous section),  $\tilde{\mu}$  is related to  $\Delta\mu$  through:

$$\Delta\mu = -\tilde{\mu} - \frac{3}{2}k_B T \ln\left(\frac{m_B}{m_A}\right). \quad (\text{S4})$$

In the VC-SGC ensemble, MC flips implemented in LAMMPS (after the modification discussed above is made) when using spatial domain decomposition are accepted with a probability of  $\min\{1, \exp(-\beta[\Delta U + \tilde{\mu}^v \Delta N_B]) \times \exp(-\frac{\kappa}{N}[(\Delta N_B)^2 + 2\Delta N_B(N_B - c_t N)])\}$ , where  $\tilde{\mu}^v$  is the average constraint parameter,  $\kappa$  is the variance constraint parameter, and  $c_t$  is the target composition. At equilibrium, the relationship with  $\Delta\mu$  is given by comparing to Eq. S3 above:

$$\Delta\mu = -\tilde{\mu}^v - 2\kappa k_B T (\langle c \rangle - c_t) - \frac{3}{2}k_B T \ln\left(\frac{m_B}{m_A}\right). \quad (\text{S5})$$

These modified equations allow the results between each ensemble to agree, as shown in Figure 2 (a) in the manuscript.

#### 4. Interfacial Widths

Figure S3 below shows the composition profile across a flat interface obtained from hybrid VC-SGC MC/molecular dynamics (MD) simulations. The solid black lines are obtained through fitting to the binned data for one of the two interfaces (two interfaces are present due to periodic boundary conditions) to Eq. 8 in the manuscript.  $l$  is found to be 0.2 nm and 0.4 nm for 600 K and 1000 K, respectively.

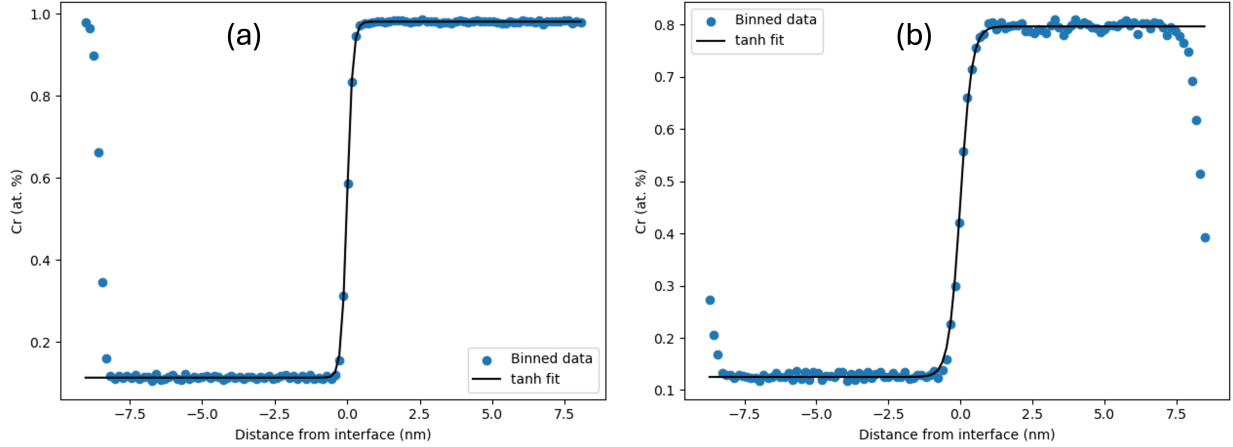

Figure S3: Compositions across an interface at (a) 600 K and (b) 1000 K where binned atomistic data is represented with blue data points and the corresponding hyperbolic tangent fit is represented with solid black lines.

## 5. Redlich-Kister Polynomial Coefficients

Table S2 shows the fitted Redlich-Kister coefficients used for modeling the excess free energy in Eq. 5 in the manuscript. These values were obtained by fitting to VC-SGC/SGC MC/MD data as discussed in the manuscript.

| coefficient (eV/atom) | 600 K                   | 1000 K                  |
|-----------------------|-------------------------|-------------------------|
| $L_0$                 | $3.374 \times 10^{-1}$  | $1.715 \times 10^{-1}$  |
| $L_1$                 | $7.843 \times 10^{-2}$  | $7.397 \times 10^{-2}$  |
| $L_2$                 | $-6.260 \times 10^{-1}$ | $1.521 \times 10^{-1}$  |
| $L_3$                 | $-5.574 \times 10^{-1}$ | $-1.944 \times 10^{-1}$ |
| $L_4$                 | $3.512 \times 10^{-1}$  | $-9.581 \times 10^{-1}$ |
| $L_5$                 | $3.042 \times 10^{-1}$  | $-6.793 \times 10^{-1}$ |
| $L_6$                 | $-5.102 \times 10^{-2}$ | $8.315 \times 10^{-1}$  |
| $L_7$                 | -                       | $9.713 \times 10^{-1}$  |
| $L_8$                 | -                       | $-2.060 \times 10^{-1}$ |
| $L_9$                 | -                       | $-3.421 \times 10^{-1}$ |

Table S2: Redlich-Kister coefficients (up to the fourth significant figure) used to model the excess free energy in this study for the Fe-Cr solid solution at 600 K and 1000 K.

## 6. Pressure Fields

Figure S4 shows a comparison of the pressure field between atomistic data and continuum model for two different cases: an  $\alpha'$  precipitate in an  $\alpha$  matrix at 600 K (a-c), and an  $\alpha$  precipitate in an  $\alpha'$  matrix at 1000 K (d-f).

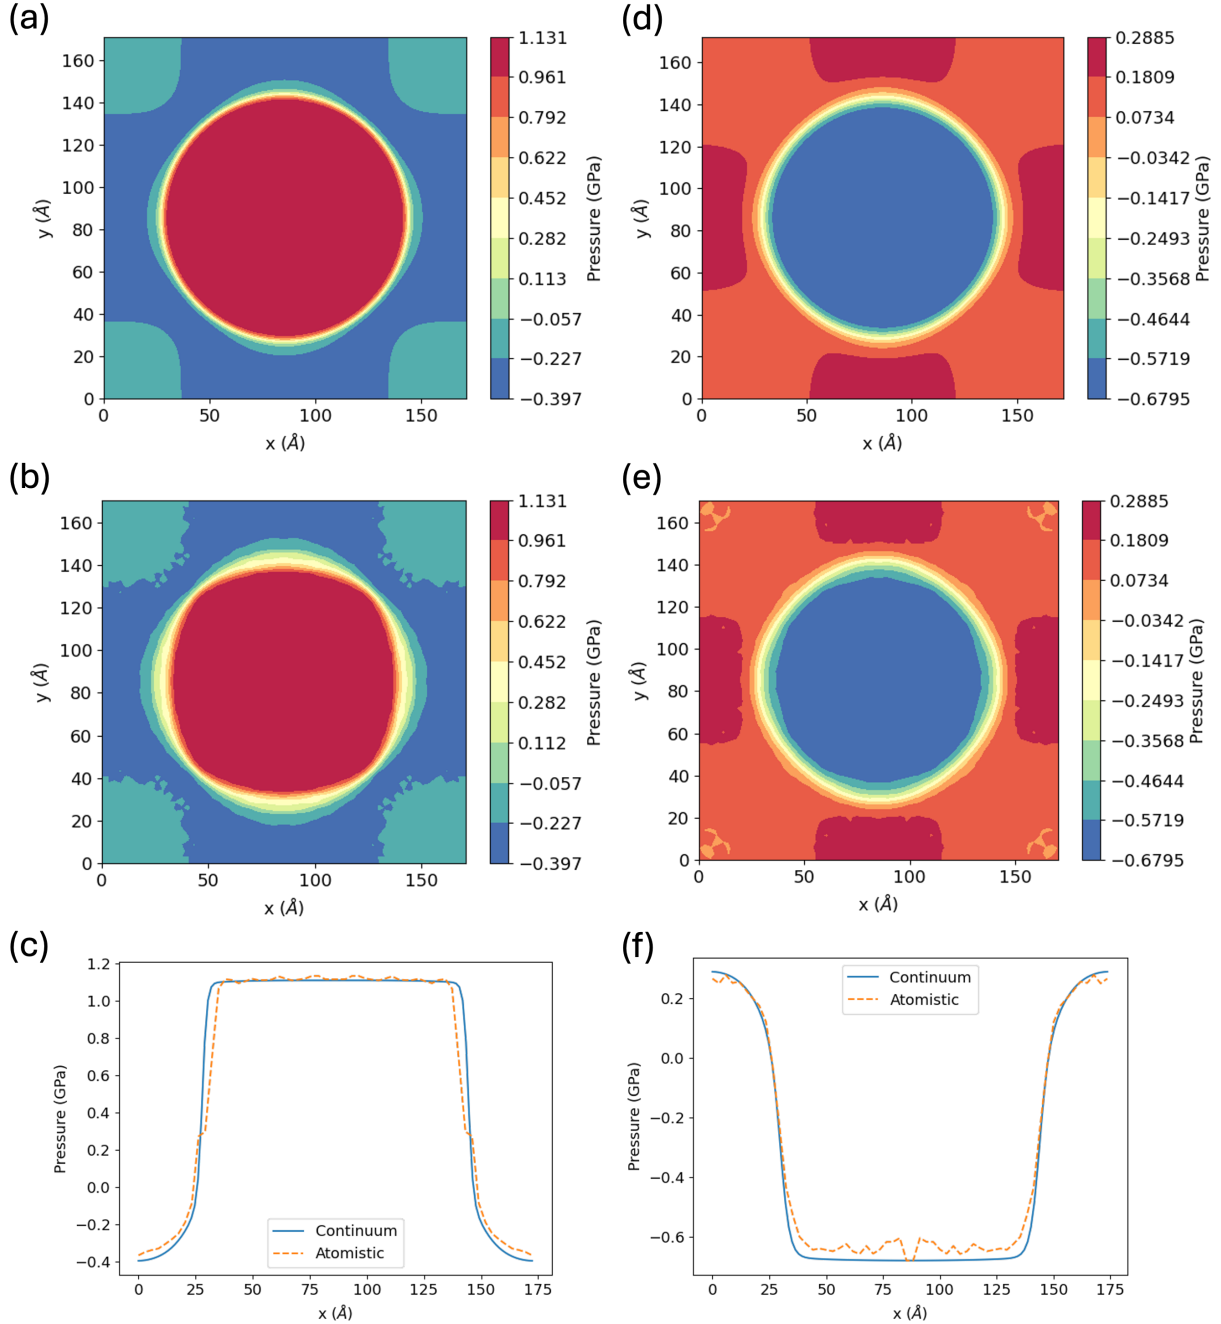

Figure S4: (a) Pressure field of an  $\alpha'$  precipitate in a  $\alpha$  matrix at 600 K from continuum modeling. (b) Same as (a) except from atomistic data. (c) Line scan across the center of the precipitate for (a) and (b). (d-f) Similar to (a-c), except for an  $\alpha$  precipitate in an  $\alpha'$  matrix at 1000 K.

## 7. von Mises Stress Fields

Figures S5, S6, and S7 show comparisons of the von Mises stress fields between atomistic data and continuum modeling for the case of an  $\alpha'$  precipitate in an  $\alpha$  matrix at 600 K, an  $\alpha$  precipitate in an  $\alpha'$  matrix at 600 K, and an  $\alpha$  precipitate in an  $\alpha'$  matrix at 1000 K, respectively. The left columns of the figures represent unfiltered data, and the right columns of the figures represent filtered data following the same procedure in the manuscript.

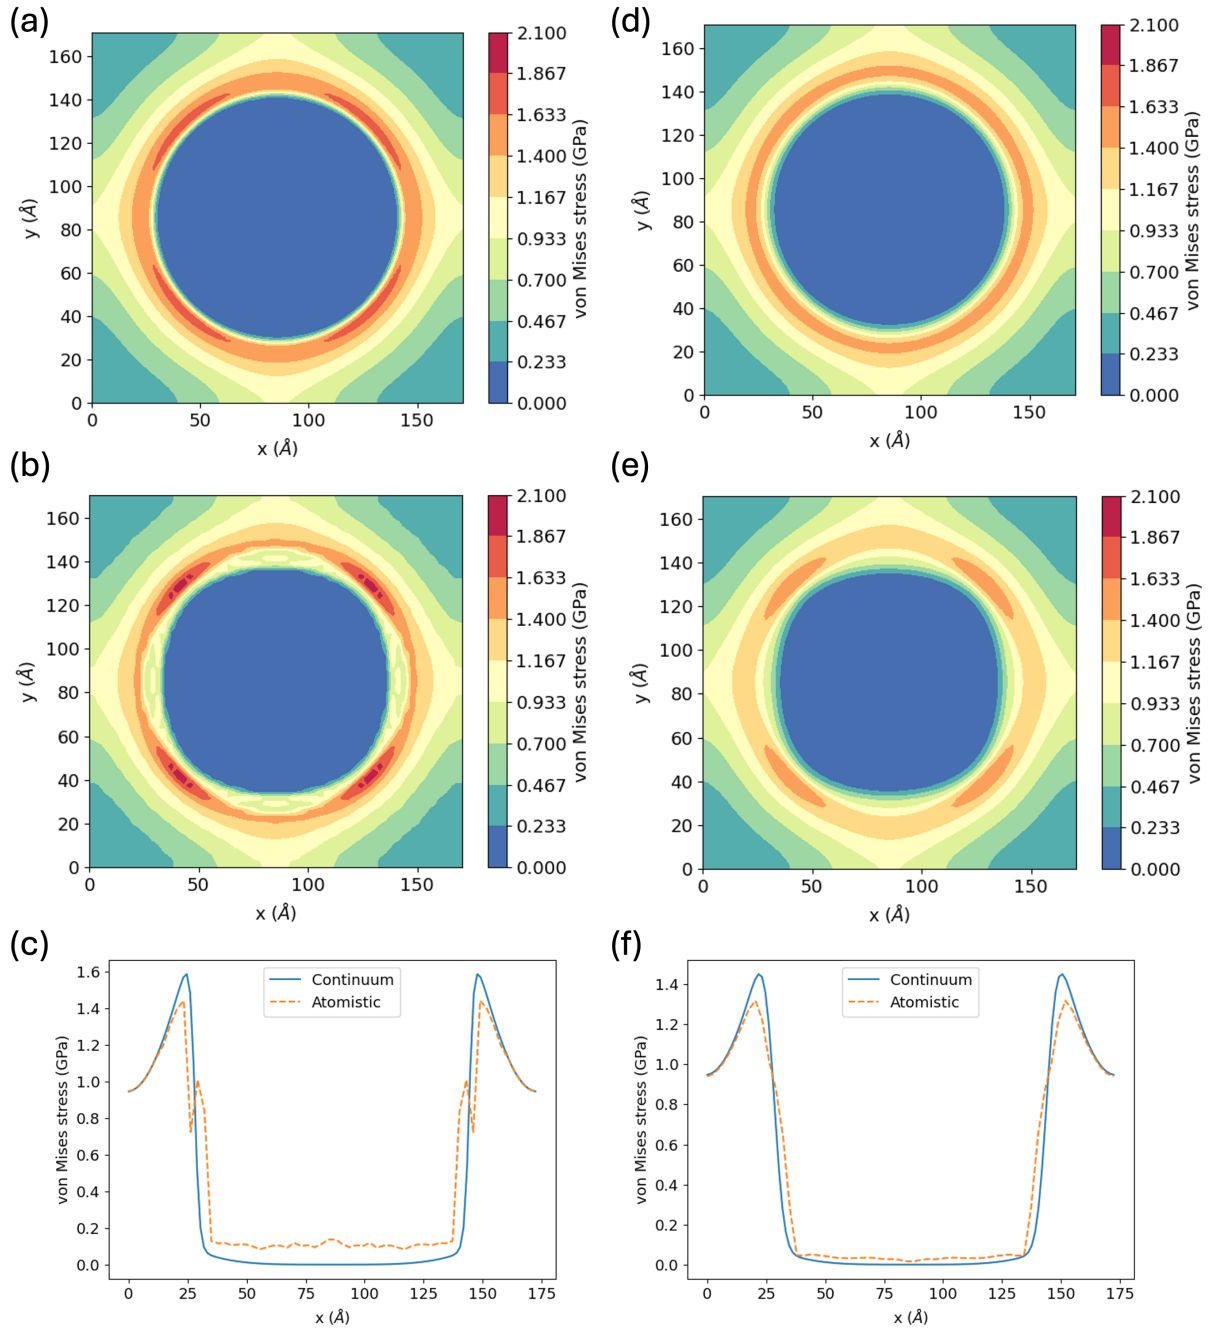

Figure S5: (a) von Mises stress field of an  $\alpha'$  precipitate in an  $\alpha$  matrix at 600 K from continuum modeling. (b) Same as (a) except from atomistic data. (c) Line scan across the center of the precipitate for (a) and (b). (d-f) Similar to (a-c), except that a Gaussian filter (with a standard deviation equal to the effective lattice constant) has been applied to the individual stress components before the von Mises stress was calculated.

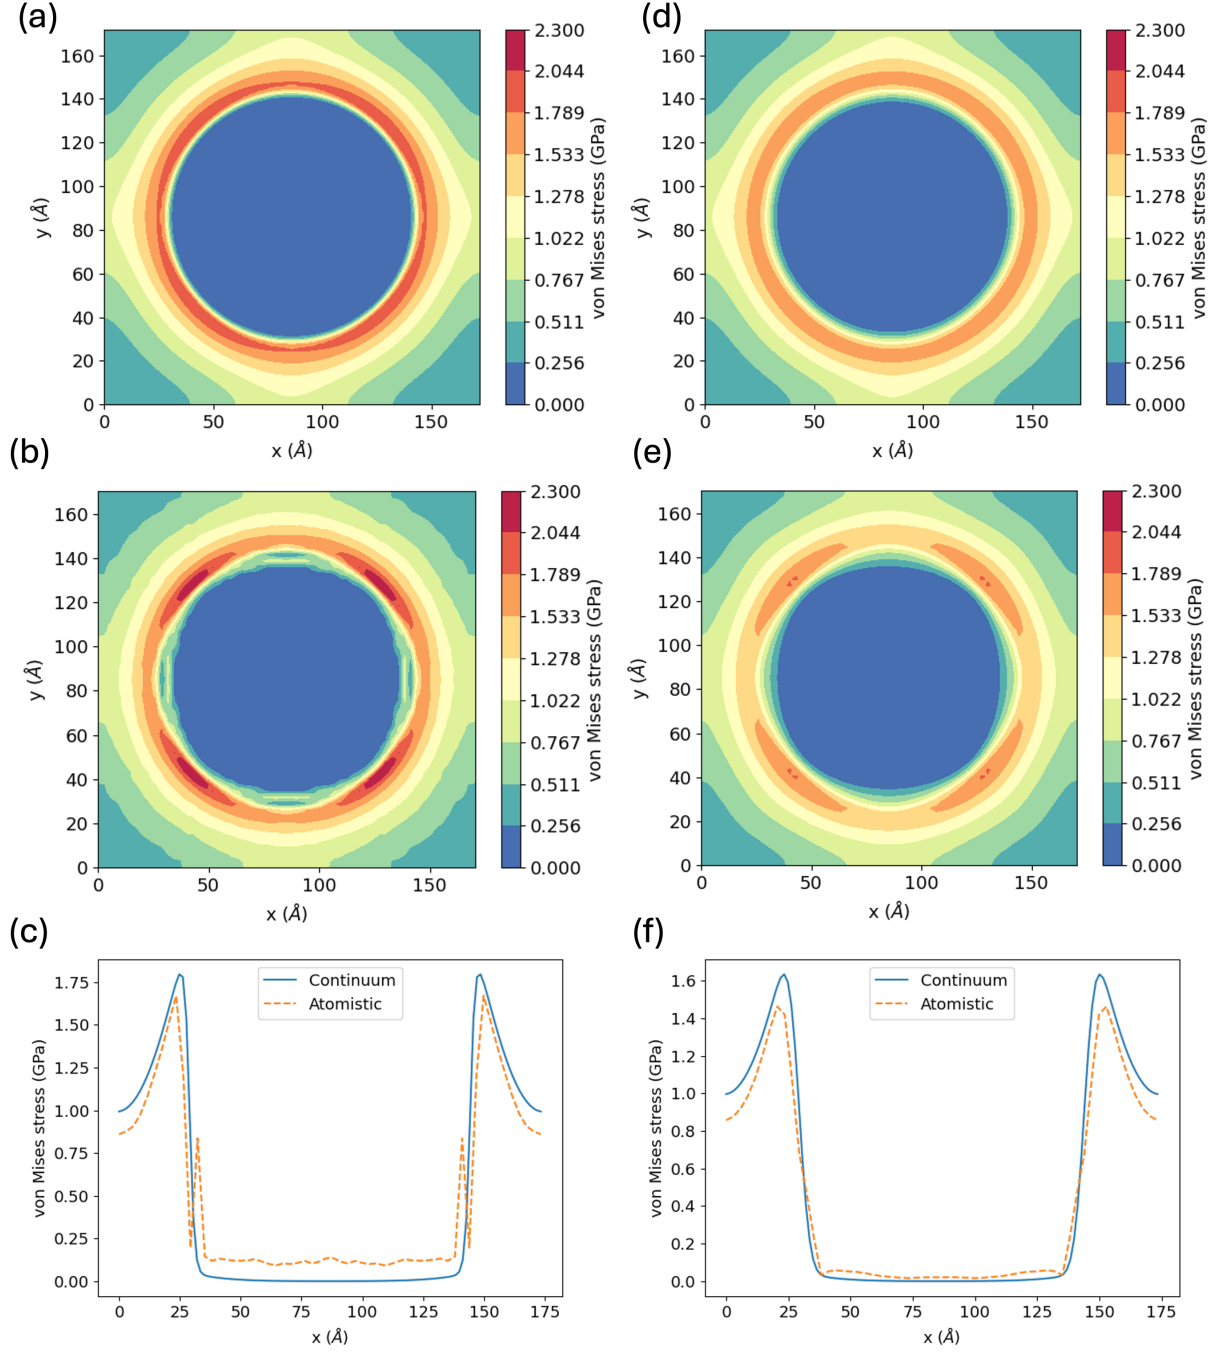

Figure S6: (a) von Mises stress field of an  $\alpha$  precipitate in an  $\alpha'$  matrix at 600 K from continuum modeling. (b) Same as (a) except from atomistic data. (c) Line scan across the center of the precipitate for (a) and (b). (d-f) Similar to (a-c), except that a Gaussian filter (with a standard deviation equal to the effective lattice constant) has been applied to the individual stress components before the von Mises stress was calculated.

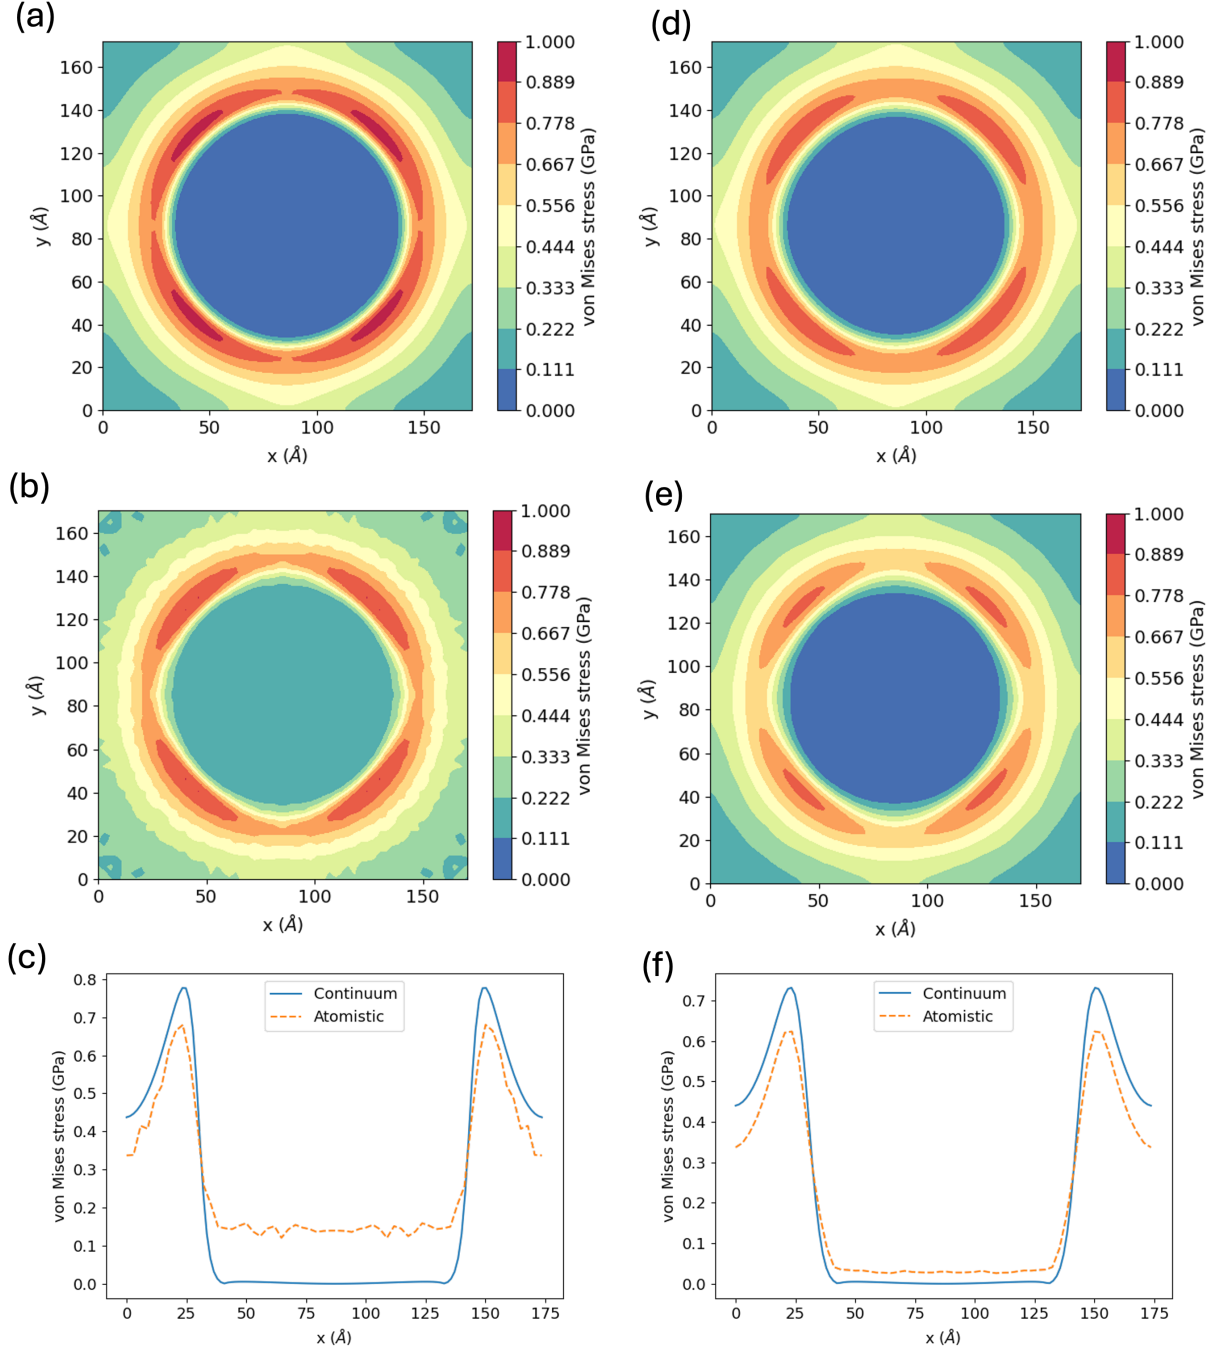

Figure S7: (a) von Mises stress field of an  $\alpha$  precipitate in an  $\alpha'$  matrix at 1000 K from continuum modeling. (b) Same as (a) except from atomistic data. (c) Line scan across the center of the precipitate for (a) and (b). (d-f) Similar to (a-c), except that a Gaussian filter (with a standard deviation equal to the effective lattice constant) has been applied to the individual stress components before the von Mises stress was calculated.

## References

- [1] A. Stukowski, B. Sadigh, P. Erhart, A. Caro, Efficient implementation of the concentration-dependent embedded atom method for molecular-dynamics and monte-carlo simulations, *Modelling and Simulation in Materials Science and Engineering* 17 (2009). doi:10.1088/0965-0393/17/7/075005.
- [2] Nist interatomic potential repository: 2009–stukowski-a-sadigh-b-erhart-p-caro-a-fe-cr, <https://www.ctcms.nist.gov/potentials/Download/2009--Stukowski-A-Sadigh-B-Erhart-P-Caro-A--Fe-Cr>.
- [3] S. M. Eich, D. Beinke, G. Schmitz, Embedded-atom potential for an accurate thermodynamic description of the iron-chromium system, *Computational Materials Science* 104 (2015) 185–192. doi:10.1016/j.commatsci.2015.03.047.
- [4] A. Caro, D. A. Crowson, M. Caro, Classical many-body potential for concentrated alloys and the inversion of order in iron-chromium alloys, *Physical Review Letters* 95 (8 2005). doi:10.1103/PhysRevLett.95.075702.
- [5] Y. Mishin, Calculation of the  $\gamma/\gamma'$  interface free energy in the ni-al system by the capillary fluctuation method, *Modelling and Simulation in Materials Science and Engineering* 22 (2014). doi:10.1088/0965-0393/22/4/045001.
- [6] Y. K. Kim, H. K. Kim, W. S. Jung, B. J. Lee, Atomistic modeling of the ti-al binary system, *Computational Materials Science* 119 (2016) 1–8. doi:10.1016/j.commatsci.2016.03.038.
- [7] Parallel grand-canonical monte carlo (paragrandmc) user’s manual version 2.0, <https://ntrs.nasa.gov/citations/20220003134>.
- [8] B. Sadigh, P. Erhart, Calculation of excess free energies of precipitates via direct thermodynamic integration across phase boundaries, *Physical Review B - Condensed Matter and Materials Physics* 86 (10 2012). doi:10.1103/PhysRevB.86.134204.
- [9] vcsgc-lammps - a monte carlo module for lammps, <https://vcsgc-lammps.materialsmodeling.org/>, accessed: 2024-07-29.
- [10] B. Sadigh, P. Erhart, A. Stukowski, A. Caro, E. Martinez, L. Zepeda-Ruiz, Scalable parallel monte carlo algorithm for atomistic simulations of precipitation in alloys, *Physical Review B - Condensed Matter and Materials Physics* 85 (5 2012). doi:10.1103/PhysRevB.85.184203.
